# Supplementary material for: Successful prediction of total $\alpha$-induced reaction cross sections at astrophysically relevant sub-Coulomb energies using a novel approach
Source: arXiv:2006.03885 ancillary file (2020-06-06)
Supplement: Supplementary file 1 [file barrier2019_supplement.pdf]

# Supplement to “Successful prediction of total $\alpha$ -induced reaction cross sections at astrophysically relevant sub-Coulomb energies using a novel approach”

P. Mohr,<sup>1,2,\*</sup> Zs. Fülöp,<sup>1</sup> Gy. Gyürky,<sup>1</sup> G. G. Kiss,<sup>1</sup> and T. Szücs<sup>1</sup>

<sup>1</sup>*Institute for Nuclear Research (MTA Atomki), H-4001 Debrecen, Hungary*

<sup>2</sup>*Diakonie-Klinikum, D-74523 Schwäbisch Hall, Germany*

(Dated: June 6, 2020)

This supplement provides more details for the calculations in the so-called pure barrier transmission model (pBTM) which are mainly addressed to experts in low-energy nuclear physics. These details have been separated from the main paper for better readability to the broad readership of Physical Review Letters. For completeness, additional references of the Supplement are listed at the end of the letter (Refs. [51–68]); all references in the Supplement are also listed at the end of the Supplement.

## I. CALCULATION OF THE ATOMKI-V1 DOUBLE-FOLDING POTENTIAL

The ATOMKI-V1 potential [1] for  $\alpha$  + nucleus is based on the analysis of  $(\alpha, \alpha)$  elastic scattering angular distributions at low energies. It consists of a real part which is derived from a double-folding procedure, and a phenomenological imaginary part of surface Woods-Saxon type. Three inputs are required for the double-folding potential: the nucleon density  $\rho_P$  of the  $\alpha$  projectile, the nucleon density  $\rho_T$  of the target nucleus, and the effective interaction  $v_{\text{eff}}$ . The density  $\rho_P$  of the  $\alpha$  projectile and the effective interaction  $v_{\text{eff}}$  are fully described in [1]. The target densities  $\rho_T$  were derived from experimental charge density distributions in [1] which were taken from the compilation of electron scattering data [2]. Such data are rare for target masses above  $A \gtrsim 150$  and not available for unstable nuclei (like the important example of  $^{176}\text{W}$ ). Consequently, the present work uses theoretical densities which were taken from the TALYS code [3]. We have chosen the microscopic Hartree-Fock-Bogolyubov densities using Skyrme forces (labeled with “Goriely” within TALYS); for stable nuclei, the resulting potentials are close to the potentials using experimental densities [2]. The sensitivity of the calculated cross sections on the chosen target density will be investigated later in Sec. VII.

From the analysis of  $(\alpha, \alpha)$  elastic scattering angular distributions it has been found in [1] that the real folding potential has to be scaled by a strength parameter  $\lambda \approx 1.2 - 1.4$ , leading to volume integrals of  $J_R \approx 330 - 410 \text{ MeV fm}^3$ . Finally, an average value of  $J_R = 342.4 \text{ MeV fm}^3$  was adopted in [1] for (semi-)magic

nuclei, and a slightly larger volume integral of  $J_R = 371.0 \text{ MeV fm}^3$  is derived for non-magic nuclei. The above procedure completely defines the calculation of the real part of the  $\alpha$ -nucleus potential and fixes all parameters which are required for the calculation of cross sections in the pBTM; there is no later adjustment of parameters to experimental (non-elastic) reaction cross sections.

## II. BARRIER TRANSMISSION MODEL AND CODE “CCFULL”

According to Eq. (2) of our paper, the cross section in the pBTM results from the transmissions  $T_L$  in a real potential which is composed of the attractive nuclear potential and the repulsive Coulomb potential. The CCFULL code [4] solves coupled channel equations for this resulting potential (see Eq. (12) of [4]) using a so-called modified Numerov method. The cross section in the simple pBTM model is calculated from the CCFULL code by switching off the couplings  $V_{nn}$  in Eq. (1) of [4]. Technically, CCFULL solves the Schrödinger equation from a minimum radius  $r_{\text{min}}$  (calculated from the Coulomb pocket inside the barrier) to a maximum radius  $r_{\text{max}}$  (where the nuclear potential is negligible). The transmissions  $T_L$  are calculated from the amplitudes of the wave function, see Eqs. (11), (16), and (17) of [4]. All details of the CCFULL code are given in [4].

The pBTM model is widely used in the fusion community. Compared to the optical model, there are several advantages. Because the pBTM does not require an imaginary part of the potential, the dramatic sensitivity of the calculated cross sections to the parameters of the imaginary potential can be completely avoided. Furthermore, for very low energies the  $T_L$  can be approximated using a semi-classical approach (typically used in  $\alpha$ -decay studies). A disadvantage of the simple pBTM is its restriction to low energies, and the pBTM can only provide total reaction cross sections  $\sigma_{\text{reac}}$ , but not partial cross sections for individual exit channels. The latter disadvantage can be overcome under certain circumstances, see Sec. V.

## III. THE ROLE OF DEFORMATION

The above ATOMKI-V1 potential and also the other widely used  $\alpha$ -nucleus optical model potentials (AOMPs) like McFadden-Satchler (MCF, [5]), Avrigeanu (AVR,

---

\* mohr@atomki.mta.hu

[6]), or Demetriou (DEM, [7]) use spherical symmetry and do not consider deformation explicitly. However, as the parameters of the different potentials are adjusted to elastic scattering and reaction cross sections, these potentials should be considered as effective potentials, and the obtained parameters are implicitly affected by deformation. For the ATOMKI-V1 potential with its few parameters this is nicely visible by the smaller volume integral  $J_R$  for semi-magic, i.e. spherical, nuclei, compared to non-magic deformed nuclei, which leads to increased cross sections for non-magic nuclei.

The transmission of  $\alpha$ -particles through deformed barriers was investigated mainly in  $\alpha$ -decay studies (e.g., [8, 9]). In general, deformation enhances the transmission by about a factor of two for quadrupole deformations  $\beta_2 \approx 0.2$ , and the enhancement does not exceed a factor of five even for very large  $\beta_2 \approx 0.3$  [10].

Fig. 4 compares the total cross sections  $\sigma_{\text{reac}}$  for  $^{176}\text{W} + \alpha$  from the volume integral  $J_R = 371 \text{ MeV fm}^3$  for deformed nuclei (this is the standard calculation, shown also in Fig. 1 of the manuscript) and from the lower volume integral  $J_R = 342.4 \text{ MeV fm}^3$  for spherical (semi-)magic nuclei. The cross section is reduced by about 30% in the Gamow window using the lower volume integral for (semi-)magic nuclei; i.e., the calculation of the cross sections for deformed non-magic nuclei is already slightly enhanced (compared to spherical nuclei). An additional artificial enhancement of the standard calculation by another factor of two (as estimated in the  $\alpha$ -decay study [10]) would – at least partly – double-count the effect of deformation and thus lead to an overestimation of the cross section.

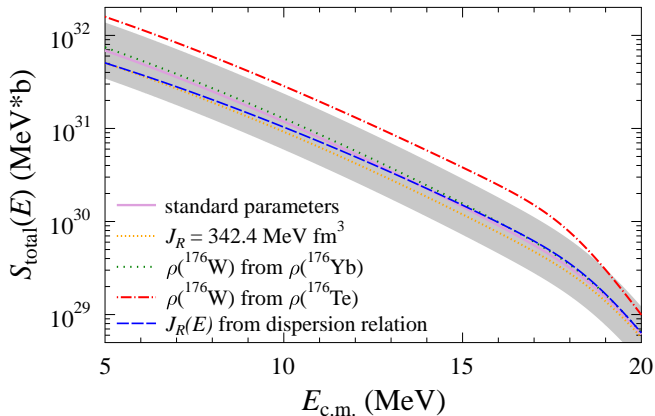

FIG. 4. (Color online) Total reaction cross section  $\sigma_{\text{reac}}$  for  $\alpha + ^{176}\text{W}$  for different potentials (shown as astrophysical  $S$ -factor). The grey-shaded area represents the estimated uncertainty of a factor of two. Further discussion see text in Sects. III, IV, and VII.

#### IV. ENERGY DEPENDENCE OF THE POTENTIAL AND DISPERSION RELATION

The full optical ATOMKI-V1 potential is comprised of an energy-independent real part and an energy-dependent imaginary part. The shapes of the real and imaginary potentials are energy-independent. These results are based on the analysis of  $(\alpha, \alpha)$  elastic scattering at energies as close as possible to the astrophysically relevant energy range; i.e., the energies for the determination of the ATOMKI-V1 potential range from slightly below the Coulomb barrier to slightly above the Coulomb barrier [1] (see also Sec. I). This energy range is experimentally challenging because high-precision data are needed to derive the optical potential from small deviations from Rutherford scattering of point-like charges.

It is well-known for a long time that the real and imaginary parts of an optical potential are coupled by a dispersion relation [11] which results from the principle of causality [12]. For simplicity, it is often assumed that the dispersion relation does not affect the radial shape of the potentials [13] which is in line with the properties of the ATOMKI-V1 potential. Thus, we use the following dispersion relation for the volume integrals  $J_R$  and  $J_I$  of the real and imaginary parts of the potential [14]:

$$\Delta J_R(E) = \frac{1}{\pi} \mathcal{P} \int_0^\infty \frac{J_I(E')}{E' - E} dE' \quad (1)$$

where  $\mathcal{P}$  denotes the principle value of the following integral, and  $\Delta J_R(E)$  is the dispersive correction to the real volume integral  $J_R$ . The integration in Eq. (1) requires the knowledge of  $J_I(E)$  for all energies from 0 to infinity. However, it has been shown that the energy dependence of  $\Delta J_R(E)$ , i.e. the shape of the dispersive correction, is well-defined from the steep increase of  $J_I(E)$  at energies around the Coulomb barrier whereas various parameterizations of the high-energy behavior of  $J_I(E)$  provide different additive corrections to  $\Delta J_R(E)$ ; this finally leads to the so-called subtracted dispersion relation [14–16].

The volume integrals  $J_R$  and  $J_I$  from the analysis of the ATOMKI-V1 potential [1] are shown as a function of the reduced energy  $E_{\text{red}}$  in Fig. 5.  $E_{\text{red}}$  is defined as [17]

$$E_{\text{red}} = \frac{(A_P^{1/3} + A_T^{1/3})E_{\text{c.m.}}}{Z_P Z_T} \quad (2)$$

which allows a simple comparison of  $J_R$  and  $J_I$  data from different nuclei; furthermore, global properties of  $J_R$  and  $J_I$  can be better identified as a function of  $E_{\text{red}}$ .

We calculated the dispersive correction  $\Delta J_R(E)$  from the imaginary volume integral of the ATOMKI-V1 potential, see Eq. (A.1) of [1] and full line in Fig. 5a, for the chosen example of  $^{176}\text{W} + \alpha$ . The resulting correction  $\Delta J_R(E)$  was adjusted by an offset to match the experimental values of  $J_R$  for non-magic nuclei. The result is shown as full line in Fig. 5b. Then, the resulting real potential with the energy-dependent  $J_R(E)$  was used to calculate the total reaction cross section  $\sigma_{\text{reac}}$  and total

S-factor for  $^{176}\text{W} + \alpha$ ; the result is included in Fig. 4 with a long-dashed blue line. The results from the dispersion relation remain close to the standard calculation with deviations below 30% in the relevant energy range in Fig. 4.

It has been pointed out (see e.g. [12]) that the consideration of the dispersion relation may enhance the cross sections around the barrier significantly; an enhancement of a factor of 50 was reported in [12]. At first view, this result seems to be in contradiction to the minor changes of less than 30% found in the present study. This contradiction is resolved by the following considerations.

Ref. [12] starts from the real part of a potential which was adjusted at higher energies far above the barrier. Indeed, under these conditions the dispersion relation leads to a significant enhancement of the real potential at ener-

gies around the barrier. Thus, the effective Coulomb barrier is reduced, and the fusion cross section is enhanced by the consideration of the dispersion relation (by the huge factor of 50 in the chosen example of  $^{16}\text{O} + ^{208}\text{Pb}$  in [12]).

Contrary, the ATOMKI-V1 potential was adjusted to elastic scattering data at energies around the Coulomb barrier, i.e. close to the energies where the maximum correction  $\Delta J_R$  from Eq. (1) is found. Thus, the major part of the dispersive correction  $\Delta J_R$  is implicitly taken into account in the ATOMKI-V1 potential, and the remaining small correction leads to a minor enhancement of the volume integral  $J_R$  by less than 10% around the maximum of the dispersive correction at about 18 MeV and to a reduction of  $J_R$  by less than 10% at astrophysically most relevant energies far below the Coulomb barrier. These minor changes of the potential by less than 10% translate to a very minor enhancement of the cross section by about 10% around 18 MeV and to a reduction of the cross section at low energies by about 15% (30%) at 10 MeV (5 MeV). These variations clearly remain within the claimed uncertainties of the present study of a factor of two.

Summarizing, the energy-independent real part of the ATOMKI-V1 potential has been derived at energies close to the Coulomb barrier. Under these special conditions, the application of the dispersion relation has only minor influence on the resulting cross sections.

For completeness it has to be mentioned that there is an additional energy dependence of the real potential which results from the energy dependence of the interaction in the folding integral. This energy dependence is small with the order of  $-0.1\%$  per MeV which is far below the effect of the dispersion relation. Consequently, the energy dependence of the interaction was neglected.

## V. DETERMINATION OF PARTIAL CROSS SECTIONS

Calculations in the pBTM can only provide the total reaction cross section  $\sigma_{\text{reac}}$ . This limitation can be overcome with the following idea. As pointed out above, the pBTM assumes absorption of the incoming  $\alpha$ -particle as soon as the  $\alpha$  has tunneled through the barrier. Such a behavior can be nicely simulated in the optical model by an imaginary part of the AOMP which is deep, narrow, and sharp-edged. By some trial and error, a standard Woods-Saxon potential with a depth  $W_0 = 50$  MeV, radius  $R_0 = 1.0$  fm,  $R = R_0 \times A_T^{1/3}$ , and diffuseness  $a = 0.10$  fm was found which is able to reproduce the  $\sigma_{\text{reac}}$  from the pBTM with minor deviations of less than 20% for all nuclei with  $A \gtrsim 50$  and for all sub-Coulomb energies. This deep, narrow, and sharp-edged imaginary potential in combination with the real part of the ATOMKI-V1 potential was implemented into TALYS. Thus, the total cross sections  $\sigma_{\text{reac}}$  from the pBTM are approximated in the TALYS calculation for the entrance

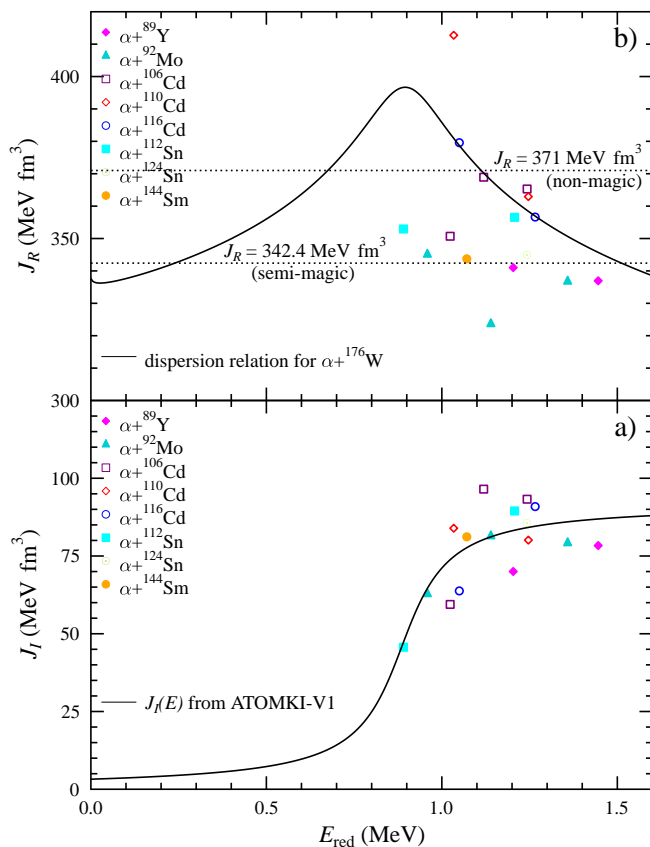

FIG. 5. (Color online) Volume integrals  $J_I$  of the imaginary part (lower diagram a) and  $J_R$  of the real part (upper diagram b) as a function of the reduced energy  $E_{\text{red}}$ . The full line for the imaginary  $J_I$  is taken from the ATOMKI-V1 potential, see Eq. (A.1) of [1]. The horizontal dotted lines for the real  $J_R$  represent the ATOMKI-V1 results for semi-magic and non-magic nuclei. The full line for  $J_R$  shows the dispersive correction  $\Delta J_R$  from  $J_I(E)$  for  $^{176}\text{W} + \alpha$  which was adjusted to the  $J_R$  for non-magic nuclei (open symbols). The range of  $E_{\text{red}}$  from 0 to 1.6 MeV corresponds to energies from 0 to about 33 MeV for the  $^{176}\text{W} + \alpha$  system. Further discussion see text.

channel, and the branchings to the different exit channels are calculated as usual in the statistical model. This potential will be called ATOMKI-V2 in the following. As an example, Fig. 6 shows the cross sections of the  $^{58}\text{Ni}(\alpha,\gamma)^{62}\text{Zn}$ ,  $^{58}\text{Ni}(\alpha,n)^{61}\text{Zn}$ , and  $^{58}\text{Ni}(\alpha,p)^{61}\text{Cu}$  reactions.

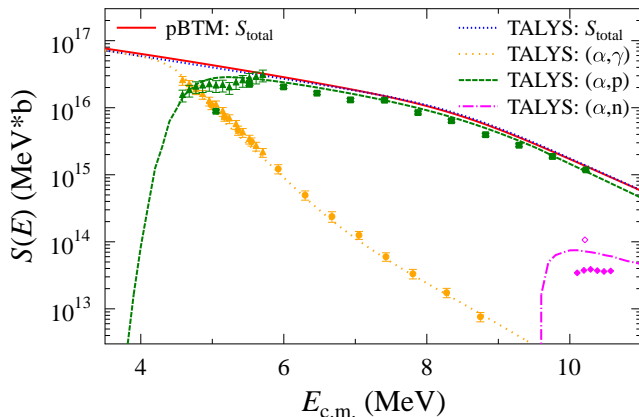

FIG. 6. (Color online)  $\alpha$ -induced cross sections for  $^{58}\text{Ni}$  (shown as astrophysical S-factors): total cross section  $\sigma_{\text{reac}}$  from the pBTM (full red line) and from TALYS using the ATOMKI-V2 potential (dotted blue line; practically identical to the pBTM, see text) and partial cross sections from TALYS with the ATOMKI-V2 potential for  $^{58}\text{Ni}(\alpha,\gamma)^{62}\text{Zn}$ ,  $^{58}\text{Ni}(\alpha,n)^{61}\text{Zn}$ , and  $^{58}\text{Ni}(\alpha,p)^{61}\text{Cu}$ , compared to the experimental data by Quinn *et al.* [18] (full circles), McGowan *et al.* [19] (full triangles), Vliks *et al.* [20] (full squares), and the contradicting early  $(\alpha,n)$  data by Cummings [21] (open diamond) and Stelson *et al.* [22] (full diamonds).

For completeness it has to be pointed out that the partial cross sections in the TALYS calculations may depend on all ingredients of the statistical model because the cross sections of  $(\alpha,X)$  reactions ( $X = p, n, \gamma, 2n$ , etc.) scale with  $T_\alpha T_X/T_{\text{tot}}$  or  $T_\alpha \times b_X$  with the transmissions  $T_i$  into the individual channels,  $T_{\text{tot}} = \sum_i T_i$ , and the branching  $b_X = T_X/T_{\text{tot}}$ . In practice, one can often identify energy ranges where one partial channel is dominating ( $b_X \approx 1$ ), and thus this dominating partial cross section fully constrains  $T_\alpha$  in the entrance channel. For  $^{58}\text{Ni}$  such a behavior is found for very low energies below 4 MeV where the  $\gamma$  channel dominates, and for energies between 6 and 10 MeV where the proton channel dominates. The calculations in Fig. 6 use the default TALYS parameters except the ATOMKI-V2 AOMP which was defined above.

## VI. APPLICABILITY OF THE PBTM IN A WIDER MASS RANGE

The present paper had a focus on heavy target nuclei in the mass region  $150 \leq A \leq 200$ . Because of the high Coulomb barrier between the incoming  $\alpha$  particle and these heavy target nuclei, any prediction of low-energy

cross sections within the OM is extremely sensitive to the tail of the imaginary part of the potential at large radii outside the colliding nuclei. Consequently, the predictions of the total  $\alpha$ -induced cross section  $\sigma_{\text{reac}}$  in the OM and the partial  $(\alpha,X)$  cross sections in the statistical model show huge discrepancies for different AOMPs; these discrepancies may reach several orders of magnitude at the astrophysically relevant sub-Coulomb energies (see Fig. 1 of the paper).

The essential role of the tail of the imaginary potential becomes less relevant for lighter target nuclei, and thus the range of predicted cross sections from different AOMPs becomes significantly smaller. For target nuclei with  $A \lesssim 50$  it was found that the simple four-parameter Woods-Saxon potential by McFadden and Satchler is able to describe the cross sections very reasonably [23]. Because of the smaller range of predictions from different AOMPs, one can expect that also the pBTM is able to reproduce  $\sigma_{\text{reac}}$  for lighter target nuclei with reasonably small deviations. This has been verified e.g. for recent data for  $^{100}\text{Mo}$  [24] and  $^{64}\text{Zn}$  [25–27]. Inspired by a new experiment by Trache [28], the calculations in the pBTM model have been extended down to  $^{58}\text{Ni}$  successfully, see Fig. 6.

The pBTM calculations were also extended towards heavier nuclei, and good agreement between the calculated cross sections for the doubly-magic  $^{208}\text{Pb}$  and semi-magic  $^{209}\text{Bi}$  nuclei and the experimental data by Barnett *et al.* [29] was found. Thus, the pBTM is able to predict total  $\alpha$ -induced reaction cross sections for stable target nuclei in a wide mass range from  $A \approx 60$  up to  $A \gtrsim 200$ . This finding holds for (semi-)magic spherical nuclei as well as for non-magic deformed nuclei (for deformation, see also Sec. III above).

## VII. APPLICABILITY OF THE PBTM BEYOND THE VALLEY OF STABILITY

Because of the lack of experimental data of  $\alpha$ -induced cross sections for heavy unstable target nuclei it is impossible to verify the pBTM predictions for nuclei outside the valley of stability. However, the pBTM is based on the transmission through the Coulomb barrier, i.e. on well-known basic physics, and thus should provide reliable predictions also beyond the valley of stability. Obviously, the pBTM predictions depend on the chosen potential which in turn depends on the densities of the target nuclei required for the calculation of the double-folding potentials. Interestingly, this sensitivity is relatively minor. Fig. 4 shows that the total cross section of  $^{176}\text{W}$  increases by about 20% when the density of the neutron-deficient unstable  $^{176}\text{W}$  is replaced by the density of the neutron-rich stable  $^{176}\text{Yb}$ . And even the density of the extremely neutron-rich dripline nucleus  $^{176}\text{Te}$  with its remarkable neutron skin results only in an increase of  $\sigma_{\text{reac}}$  by about a factor of two. For information, the root-mean-square radii of the proton, neutron, and total densities of  $^{176}\text{W}$ ,

$^{176}\text{Yb}$ , and  $^{176}\text{Te}$  are listed in Table II.

TABLE II. Root-mean-square radii  $r_{\text{rms}}$  of the proton, neutron, and total nucleon densities for  $A = 176$  nuclei from the TALYS database. All values are given in fm.

| nucleus           | $Z$ | $N$ | $r_{\text{rms}}(\text{p})$ | $r_{\text{rms}}(\text{n})$ | $r_{\text{rms}}(\text{total})$ |
|-------------------|-----|-----|----------------------------|----------------------------|--------------------------------|
| $^{176}\text{W}$  | 74  | 102 | 5.207                      | 5.285                      | 5.253                          |
| $^{176}\text{Yb}$ | 70  | 106 | 5.180                      | 5.321                      | 5.265                          |
| $^{176}\text{Te}$ | 52  | 124 | 5.051                      | 5.544                      | 5.403                          |

From the relatively minor sensitivity to the chosen density we think that the claimed uncertainty for the total cross sections of a factor of two also holds for the unstable target nuclei which are relevant for  $p$ -process nucleosynthesis. Note that the  $p$ -process path is located relatively close to stability in the  $A \approx 100$  mass region and a few mass units “west” of stability for heavy  $p$ -nuclei. Similar uncertainties of about a factor of two are also expected for the weak  $r$ -process where  $(\alpha, n)$  reactions on neutron-rich nuclei may be faster than  $\beta$ -decay for the production of nuclei with increasing  $Z$  [30–33].

There are ongoing experiments of  $\alpha$ -induced cross sections for the unstable target nuclei  $^{75}\text{Ga}$  and  $^{85}\text{Br}$  at NSCL [34] and for  $^{106}\text{Mo}$  at ANL [35]. Our predictions from the pBTM were sent to both groups, and we hope that a comparison between our predictions and the new experimental data will become possible within the near future. In general, the predictions from the pBTM should be at least as reliable as the predictions from the many-parameter AOMPs where the  $N$ ,  $Z$ , and  $A$  dependence of the AOMP is only constrained for stable target nuclei, and the resulting extrapolation to unstable target nuclei may be very uncertain.

### VIII. ASTROPHYSICAL REACTION RATES

The astrophysical reaction rates  $N_A \langle \sigma v \rangle$  are shown in Fig. 3 of the main paper. Obviously, the rates from literature show a wide range of predicted  $N_A \langle \sigma v \rangle$  of several orders of magnitude whereas the present approach should be valid within an uncertainty of a factor of two.

The reaction rates from the REACLIB library [36] are based on the calculations by Rauscher and Thielemann [37] which in turn are based on the AOMP by MCF. It turns out that the REACLIB rates are higher than the present result by more than one order magnitude which

is even beyond the range of variations in the sensitivity study [38]. However, there is a steep drop for low temperatures. Surprisingly, the rate from TALYS using the same AOMP by MCF leads to rates which are much higher by at least one order of magnitude than the REACLIB rate below  $T_9 \approx 3$ .

The reaction rates in the STARLIB library [39] are based on the AOMP by Demetriou (version 3) and have been calculated using an earlier TALYS version. A repetition of this calculation using the latest TALYS version 1.9 shows slightly higher rates at low and at high temperatures. These findings clearly indicate that the calculation of  $\alpha$ -induced reaction rates in the SM is also numerically very delicate.

The new rate from the pBTM is close to the TALYS rate using the Demetriou AOMP at temperatures above  $T_9 \approx 2$ ; however, at lower temperatures the present result is much lower, reaching a discrepancy of two orders of magnitude at  $T_9 \approx 1$ . The many-parameter AOMP by Avrigeanu *et al.* [6] predicts higher rates by about one order of magnitude. The simple WS potential by McFadden and Satchler exceeds the present calculation in the pBTM by several orders of magnitude.

Because of the excellent reproduction of the energy dependence of the astrophysical S-factor for many target nuclei in the pBTM (see Fig. 2 of the main paper) and because the deviations of the absolute S-factors are below a factor of two, we claim that the predicted rate from the pBTM should be reliable within a factor of two. The new rates are listed for several temperatures in Table III. In addition, the energy  $E_0$  of the classical Gamow window is provided. Because of the increasing S-factor towards lower energies, the effective Gamow window  $E_0^{\text{eff}}$  is slightly shifted towards lower energies (as e.g. discussed in [40]).

TABLE III. Astrophysical reaction rate  $N_A \langle \sigma v \rangle$  for the  $^{176}\text{W}(\alpha, \gamma)^{180}\text{Os}$  reaction from the pBTM.

| $T_9$ | $E_0$ (MeV) | $E_0^{\text{eff}}$ (MeV) | $N_A \langle \sigma v \rangle$ ( $\text{cm}^3 \text{s}^{-1} \text{mole}^{-1}$ ) |
|-------|-------------|--------------------------|---------------------------------------------------------------------------------|
| 1.5   | 7.0         | 6.8                      | $6.1 \times 10^{-30}$                                                           |
| 2.0   | 8.5         | 8.1                      | $9.4 \times 10^{-24}$                                                           |
| 2.5   | 9.9         | 9.3                      | $2.1 \times 10^{-19}$                                                           |
| 3.0   | 11.2        | 10.3                     | $3.9 \times 10^{-16}$                                                           |
| 3.5   | 12.4        | 11.3                     | $1.5 \times 10^{-13}$                                                           |

- [1] P. Mohr, G. Kiss, Z. Fülöp, D. Galaviz, G. Gyürky, and E. Somorjai, Atomic Data and Nuclear Data Tables **99**, 651 (2013).  
[2] H. D. Vries, C. D. Jager, and C. D. Vries, Atomic Data and Nuclear Data Tables **36**, 495 (1987).

- [3] A. J. Koning, S. Hilaire, and S. Goriely, “computer code TALYS, version 1.9,” (2017).  
[4] K. Hagino, N. Rowley, and A. Kruppa, Computer Physics Communications **123**, 143 (1999).  
[5] L. McFadden and G. R. Satchler, Nuclear Physics **84**,

- 177 (1966).
- [6] V. Avrigeanu, M. Avrigeanu, and C. Măniilescu, *Phys. Rev. C* **90**, 044612 (2014).
  - [7] P. Demetriou, C. Grama, and S. Goriely, *Nuclear Physics A* **707**, 253 (2002).
  - [8] D. S. Delion, Z. Ren, A. Dumitrescu, and D. Ni, *Journal of Physics G: Nuclear and Particle Physics* **45**, 053001 (2018).
  - [9] C. Xu and Z. Ren, *Phys. Rev. C* **73**, 041301 (2006).
  - [10] D. S. Delion, A. Sandulescu, and W. Greiner, *Phys. Rev. C* **69**, 044318 (2004).
  - [11] H. Feshbach, *Ann. Phys. (N.Y.)* **5**, 357 (1958).
  - [12] M. A. Nagarajan, C. C. Mahaux, and G. R. Satchler, *Phys. Rev. Lett.* **54**, 1136 (1985).
  - [13] M. A. Nagarajan and G. R. Satchler, *Physics Letters B* **173**, 29 (1986).
  - [14] C. Mahaux, H. Ngô, and G. R. Satchler, *Nuclear Physics A* **449**, 354 (1986).
  - [15] C. Mahaux, H. Ngô, and G. R. Satchler, *Nuclear Physics A* **456**, 134 (1986).
  - [16] H. Abele and G. Staudt, *Phys. Rev. C* **47**, 742 (1993).
  - [17] P. R. S. Gomes, J. Lubian, I. Padron, and R. M. Anjos, *Phys. Rev. C* **71**, 017601 (2005).
  - [18] S. J. Quinn, A. Spyrou, E. Bravo, T. Rauscher, A. Simon, A. Battaglia, M. Bowers, B. Bucher, C. Casarella, M. Couder, P. A. DeYoung, A. C. Dombos, J. Görres, A. Kontos, Q. Li, A. Long, M. Moran, N. Paul, J. Pereira, D. Robertson, K. Smith, M. K. Smith, E. Stech, R. Talwar, W. P. Tan, and M. Wiescher, *Phys. Rev. C* **89**, 054611 (2014).
  - [19] F. K. McGowan, P. H. Stelson, and W. G. Smith, *Phys. Rev.* **133**, B907 (1964).
  - [20] A. Vlieks, J. Morgan, and S. Blatt, *Nuclear Physics A* **224**, 492 (1974).
  - [21] J. B. Cumming, *Phys. Rev.* **114**, 1600 (1959).
  - [22] P. H. Stelson and F. K. McGowan, *Phys. Rev.* **133**, B911 (1964).
  - [23] P. Mohr, *The European Physical Journal A* **51**, 56 (2015).
  - [24] T. N. Szegedi, G. G. Kiss, G. Gyürky, and P. Mohr, “Activation cross section measurement of the  $^{100}\text{Mo}(\alpha, n)^{103}\text{Ru}$  reaction for optical potential studies,” (2019), *proc. Nuclear Physics in Astrophysics NPA-IX*, *J. Phys. Conf. Proc.*, accepted for publication.
  - [25] G. Gyürky, P. Mohr, Z. Fülöp, Z. Halász, G. G. Kiss, T. Szücs, and E. Somorjai, *Phys. Rev. C* **86**, 041601 (2012).
  - [26] A. Ornelas, P. Mohr, G. Gyürky, Z. Elekes, Z. Fülöp, Z. Halász, G. G. Kiss, E. Somorjai, T. Szücs, M. P. Takács, D. Galaviz, R. T. Güray, Z. Korkulu, N. Özkan, and C. Yalçın, *Phys. Rev. C* **94**, 055807 (2016).
  - [27] P. Mohr, G. Gyürky, and Z. Fülöp, *Phys. Rev. C* **95**, 015807 (2017).
  - [28] L. Trache, *EPJ Web Conf.* **227**, 01016 (2020).
  - [29] A. R. Barnett and J. S. Lilley, *Phys. Rev. C* **9**, 2010 (1974).
  - [30] J. Bliss, A. Arcones, F. Montes, and J. Pereira, *Phys. Rev. C* **101**, 055807 (2020).
  - [31] J. Bliss, A. Arcones, F. Montes, and J. Pereira, *Journal of Physics G: Nuclear and Particle Physics* **44**, 054003 (2017).
  - [32] J. Pereira and F. Montes, *Phys. Rev. C* **93**, 034611 (2016).
  - [33] P. Mohr, *Phys. Rev. C* **94**, 035801 (2016).
  - [34] J. Pereira, private communication (2019).
  - [35] M. Avila, private communication (2019).
  - [36] R. H. Cyburt, A. M. Amthor, R. Ferguson, Z. Meisel, K. Smith, S. Warren, A. Heger, R. D. Hoffman, T. Rauscher, A. Sakharuk, H. Schatz, F. K. Thielemann, and M. Wiescher, *The Astrophysical Journal Supplement Series* **189**, 240 (2010).
  - [37] T. Rauscher and F.-K. Thielemann, *Atomic Data and Nuclear Data Tables* **75**, 1 (2000).
  - [38] T. Rauscher, N. Nishimura, R. Hirschi, G. Cescutti, A. S. J. Murphy, and A. Heger, *Mon. Not. R. Astron. Soc.* **463**, 4153 (2016).
  - [39] A. L. Sallaska, C. Iliadis, A. E. Champagne, S. Goriely, S. Starrfield, and F. X. Timmes, *The Astrophysical Journal Supplement Series* **207**, 18 (2013).
  - [40] T. Rauscher, *Phys. Rev. C* **81**, 045807 (2010).
